# Supplementary material for: Dress-Me-Up: A Dataset & Method for Self-Supervised 3D Garment Retargeting
Source: arXiv:2401.03108 source file (2024-01-06)
Supplement: Supplementary file 1 [file m3dvton.tex]

\begin{figure*}
    \begin{tikzpicture}[scale=0.9]
    \node (A) at (-.5,0) {\includegraphics[width=1.05\textwidth]{assets/images/suppl_figures/m3dvton/m3dvton_comp1.png}};
    \node (B) at (0,-10) {\includegraphics[width=\textwidth, trim={0 0 0 12cm},clip]{assets/images/suppl_figures/m3dvton/m3dvton_comp2.png}};
    \end{tikzpicture}
    \caption{The figure shows retargeting results on images of MPV3D\cite{M3DVTON} against the results obtained by M3DVTON. Please observe the geometric inconsistencies in the results of M3DVTON despite having simple garment structures}
    \label{fig:m3dvton}
\end{figure*}
