# Supplementary material for: Dress-Me-Up: A Dataset & Method for Self-Supervised 3D Garment Retargeting
Source: arXiv:2401.03108 source file (2024-01-06)
Supplement: Supplementary file 2 [file wrinkle_generation_pipeline.tex]

\begin{figure}
    \includegraphics[width=\linewidth]{assets/images/suppl_figures/wrinkle_generation/wrinkle_gen.png};
    \caption{Pipeline Diagram for Wrinkle generation}
    \label{fig:wrinkle_generation}
\end{figure}
